# Supplementary material for: Facial Reenactment Through a Personalized Generator
Source: arXiv:2307.06307 source file (2023-07-12)
Supplement: Supplementary file 1 [file supp.tex]

\documentclass[acmtog,anonymous,review]{acmart}
\acmSubmissionID{237}

\citestyle{acmauthoryear}

\input{packages}
\input{macros}

\SetAlFnt{\small}
\SetAlCapFnt{\small}
\SetAlCapNameFnt{\small}
\SetAlCapHSkip{0pt}

\makeatletter
\newcommand*{\addFileDependency}[1]{%
  \typeout{(#1)}
  \@addtofilelist{#1}
  \IfFileExists{#1}{}{\typeout{No file #1.}}
}
\makeatother

\newcommand*{\myexternaldocument}[1]{%
    \externaldocument{#1}%
    \addFileDependency{#1.tex}%
    \addFileDependency{#1.aux}%
}

\myexternaldocument{main}

\acmJournal{TOG}

\begin{document}
\title{Facial Reenactment Through a Personalized Generator}

\begin{CCSXML}
<ccs2012>
   <concept>
       <concept_id>10010147.10010371.10010382</concept_id>
       <concept_desc>Computing methodologies~Image manipulation</concept_desc>
       <concept_significance>500</concept_significance>
       </concept>
 </ccs2012>
\end{CCSXML}

\ccsdesc[500]{Computing methodologies~Image manipulation -- Appendices}

\keywords{Personalization, Facial Reenactment.}

\maketitle

\appendix
\input{sections/appendices}

\newpage

{
\small
\bibliographystyle{ACM-Reference-Format}
\bibliography{main}
}

\end{document}
